# Supplementary material for: Finding Meaningful Distributions of ML Black-boxes under Forensic Investigation
Source: arXiv:2305.05869 source file (2023-05-10)
Supplement: Supplementary file 1 [file appendix.tex]

\appendix
\section{CIFAR-100}

\begin{table}[H]
\centering
\setlength{\tabcolsep}{0.5pt}
\begin{tabular}{|c|c|c|c|c|} 
\hline
                                                                        & \textbf{Victim } & \begin{tabular}[c]{@{}c@{}}\textbf{Clone}\\\textbf{CIFAR100 }\end{tabular} & \begin{tabular}[c]{@{}c@{}}\textbf{Clone}\\\textbf{Caltech101 }\end{tabular} & \begin{tabular}[c]{@{}c@{}}\textbf{Clone}\\\textbf{Flowers }\end{tabular}  \\ 
\hline
\begin{tabular}[c]{@{}c@{}}aquatic \\mammals\end{tabular}               & 61.6\%           & 37.2\%                                                                     & 14.6\%                                                                       & 6.0\%                                                                      \\ 
\hline
fish                                                                    & 75.4\%           & 48.8\%                                                                     & 16.2\%                                                                       & 10.2\%                                                                     \\ 
\hline
flowers                                                                 & 81.6\%           & 61.4\%                                                                     & 8.0\%                                                                        & 11.6\%                                                                     \\ 
\hline
\begin{tabular}[c]{@{}c@{}}food \\containers\end{tabular}               & 74.2\%           & 47.2\%                                                                     & 8.0\%                                                                        & 0.0\%                                                                      \\ 
\hline
\begin{tabular}[c]{@{}c@{}}fruit and \\vegetables\end{tabular}          & 83.8\%           & 63.6\%                                                                     & 6.6\%                                                                        & 8.8\%                                                                      \\ 
\hline
\begin{tabular}[c]{@{}c@{}}household \\electrical device\end{tabular}   & 79.6\%           & 52.6\%                                                                     & 17.2\%                                                                       & 6.8\%                                                                      \\ 
\hline
\begin{tabular}[c]{@{}c@{}}household\\furniture\end{tabular}            & 81.6\%           & 59.4\%                                                                     & 34.8\%                                                                       & 17.6\%                                                                     \\ 
\hline
insects                                                                 & 77.4\%           & 52.2\%                                                                     & 26.8\%                                                                       & 20.2\%                                                                     \\ 
\hline
\begin{tabular}[c]{@{}c@{}}large \\carnivores\end{tabular}              & 77.6\%           & 53.0\%                                                                     & 17.0\%                                                                       & 7.8\%                                                                      \\ 
\hline
\begin{tabular}[c]{@{}c@{}}large man-made\\outdoor things\end{tabular}  & 87.0\%           & 70.0\%                                                                     & 42.6\%                                                                       & 20.2\%                                                                     \\ 
\hline
\begin{tabular}[c]{@{}c@{}}large natural\\outdoor scenes\end{tabular}   & 85.0\%           & 68.6\%                                                                     & 69.0\%                                                                       & 60.0\%                                                                     \\ 
\hline
\begin{tabular}[c]{@{}c@{}}large omnivores\\and herbivores\end{tabular} & 78.4\%           & 48.6\%                                                                     & 5.4\%                                                                        & 1.2\%                                                                      \\ 
\hline
\begin{tabular}[c]{@{}c@{}}medium-sized\\mammals\end{tabular}           & 77.8\%           & 47.6\%                                                                     & 2.8\%                                                                        & 0.0\%                                                                      \\ 
\hline
\begin{tabular}[c]{@{}c@{}}non-insect\\invertebrates\end{tabular}       & 76.8\%           & 41.6\%                                                                     & 20.6\%                                                                       & 5.2\%                                                                      \\ 
\hline
people                                                                  & 54.2\%           & 36.2\%                                                                     & 5.4\%                                                                        & 1.0\%                                                                      \\ 
\hline
reptiles                                                                & 63.8\%           & 33.8\%                                                                     & 12.8\%                                                                       & 3.2\%                                                                      \\ 
\hline
\begin{tabular}[c]{@{}c@{}}small \\mammals\end{tabular}                 & 64.4\%           & 33.0\%                                                                     & 0.4\%                                                                        & 0.0\%                                                                      \\ 
\hline
trees                                                                   & 76.0\%           & 55.8\%                                                                     & 20.2\%                                                                       & 5.2\%                                                                      \\ 
\hline
vehicles 1                                                              & 86.6\%           & 59.2\%                                                                     & 13.4\%                                                                       & 0.0\%                                                                      \\ 
\hline
vehicles 2                                                              & 86.0\%           & 65.0\%                                                                     & 17.6\%                                                                       & 5.8\%                                                                      \\ 
\hline
\textbf{Average }                                                       & \textbf{76.44\% } & \textbf{51.74\% }                                                          & \textbf{17.97\% }                                                            & \textbf{9.54\% }                                                           \\
\hline
\end{tabular}
\end{table}

\begin{table}[H]
\centering
\begin{tabular}{|c|c|l|l|} 
\hline
                                                                        & \textbf{Victim }  & \textbf{Basic}   & \textbf{filter}   \\ 
\hline
\begin{tabular}[c]{@{}c@{}}aquatic \\mammals\end{tabular}               & 61.6\%            & 32.2\%           & 30.2\%            \\ 
\hline
fish                                                                    & 75.4\%            & 28.0\%           & 33.6\%            \\ 
\hline
flowers                                                                 & 81.6\%            & 29.4\%           & 34.2\%            \\ 
\hline
\begin{tabular}[c]{@{}c@{}}food \\containers\end{tabular}               & 74.2\%            & 36.4\%           & 40.8\%            \\ 
\hline
\begin{tabular}[c]{@{}c@{}}fruit and \\vegetables\end{tabular}          & 83.8\%            & 52.8\%           & 47.6\%            \\ 
\hline
\begin{tabular}[c]{@{}c@{}}household \\electrical device\end{tabular}   & 79.6\%            & 47.2\%           & 47.0\%            \\ 
\hline
\begin{tabular}[c]{@{}c@{}}household\\furniture\end{tabular}            & 81.6\%            & 53.8\%           & 50.2\%            \\ 
\hline
insects                                                                 & 77.4\%            & 39.4\%           & 40.8\%            \\ 
\hline
\begin{tabular}[c]{@{}c@{}}large \\carnivores\end{tabular}              & 77.6\%            & 46.4\%           & 52.2\%            \\ 
\hline
\begin{tabular}[c]{@{}c@{}}large man-made\\outdoor things\end{tabular}  & 87.0\%            & 56.8\%           & 56.2\%            \\ 
\hline
\begin{tabular}[c]{@{}c@{}}large natural\\outdoor scenes\end{tabular}   & 85.0\%            & 63.0\%           & 57.4\%            \\ 
\hline
\begin{tabular}[c]{@{}c@{}}large omnivores\\and herbivores\end{tabular} & 78.4\%            & 45.0\%           & 46.6\%            \\ 
\hline
\begin{tabular}[c]{@{}c@{}}medium-sized\\mammals\end{tabular}           & 77.8\%            & 28.4\%           & 39.2\%            \\ 
\hline
\begin{tabular}[c]{@{}c@{}}non-insect\\invertebrates\end{tabular}       & 76.8\%            & 39.44\%          & 39.2\%            \\ 
\hline
people                                                                  & 54.2\%            & 21.6\%           & 28.2\%            \\ 
\hline
reptiles                                                                & 63.8\%            & 25.2\%           & 22.0\%            \\ 
\hline
\begin{tabular}[c]{@{}c@{}}small \\mammals\end{tabular}                 & 64.4\%            & 27.0\%           & 30.4\%            \\ 
\hline
trees                                                                   & 76.0\%            & 24.8\%           & 31.2\%            \\ 
\hline
vehicles 1                                                              & 86.6\%            & 54.2\%           & 56.2\%            \\ 
\hline
vehicles 2                                                              & 86.0\%            & 64.4\%           & 53.6\%            \\ 
\hline
\textbf{Average }                                                       & \textbf{76.44\% } & \textbf{40.77\%} & \textbf{41.88\%}  \\
\hline
\end{tabular}
\end{table}
